# Supplementary material for: Quantifying Privacy Risks of Masked Language Models Using Membership Inference Attacks
Source: arXiv:2203.03929 source file (2022-11-04)
Supplement: Supplementary file 1 [file appendix.tex]

\section{Appendix}

%%%%%%%%
\begin{table}[]
    \centering
    % \footnotesize
    % \fontsize{7}{7}
%    \renewcommand{\arraystretch}{0.6}
    \caption{Summary of our attack's notation.}
    \vspace{-2ex}
    \label{tab:attack_notation}
    \begin{adjustbox}{width=0.65
    \linewidth, center}
    \input{tables/attack_notation}
    \end{adjustbox}
\end{table}
%%%%%%%%

\begin{table*}[]
    \centering
    % \footnotesize
    % \fontsize{7}{7}
%    \renewcommand{\arraystretch}{0.6}
    \caption{Breakdown of the sample-level attack on four different ClinicalBERT models, using PubMed-BERT as the reference. Sample-level attack attempts to determine the membership of a single sample. In this table, the MIMIC-III held-out data is used as non-members in the target sample pool.}
    \vspace{-2ex}
    \label{tab:app:sample-out-len}
    \begin{adjustbox}{width=\textwidth, center}
     \newcolumntype{L}{>{\RaggedLeft\arraybackslash}p{0.06\linewidth}} 
  \newcolumntype{O}{>{\RaggedLeft\arraybackslash}m{0.07\linewidth}} 
  \newcolumntype{D}{>{\arraybackslash}m{0.15\linewidth}} 
  \newcolumntype{R}{>{\arraybackslash}m{0.29\linewidth}} 
% \begin{tabular}{@{}cDrrrrrcrrrr@{}}
\begin{tabular}{@{}clSSSSScSSSSS@{}}
	\toprule
	& {\multirow{2}{*}{}} &  \multicolumn{4}{c}{{Short}}&{}& \multicolumn{4}{c}{{Long}}   \\
	\cmidrule{3-6} \cmidrule{8-11}
	&   &  {Base} & {Long} &  {Large} &{Large++}& {} & {Base} &{Long} & {Large}& {Large++}  \\
% 	&Metric &Original &A4NT	&One-LM	 &One-LM (DB25)	 &One-LM (DB40)	 &Inters.	&Inters. (DB25)	&Inters. (DB40)	&Union \\
	%%%%%%%%%
    \midrule
	%%%%%%%%%
    \multirow{2}{*}{\STAB{AUC.}} 
    &Baseline   & 51.6&	51.3&	50.9&	53.6&	&66.2&	65.6&	67.9&	70.0	\\
    &Ours	    & 83.0&	82.7&	83.5&	84.3&	&90.0&	89.4&	90.4&	90.5   \\
    %%%%%%%%%%&&&&&&&\\&&&&      &  & & &&&&&& &  & & && & &
           \midrule[0.1pt]
    \multirow{2}{*}{\STAB{Prec.}}
    &Baseline	& 50.9&	50.6&	50.7&	52.5&	&61.5&	61.1&	62.5&	65.0   \\
    &Baseline 2 & 48.3&	47.9&	48.1&	51.0&	&61.5&	61.6&	63.9&	66.1 \\ 
    &Ours	    & 97.2&	97.5&	97.1&	96.2&	&99.0&	99.0&	98.9&	98.1   \\
    %%%%%%%%%%%&&&&&&&\\&&&&     &  & & &&&&&& &  & & && & &
           \midrule[0.1pt]
    \multirow{2}{*}{\STAB{Acc.}}
    &Baseline	&   55.4&	55.2&	56.1&	55.9&	&54.8&	54.8&	55.0&	55.4  \\
    &Baseline 2 &   26.2&	25.4&	28.3&	31.5&	&37.9&	38.2&	43.4&	48.8 \\
    &Ours	    &   44.1&	43.4&	46.0&	48.2&	&50.9&	50.2&	52.5&	55.0   \\
    %%%%%%%%%%%&&&&&&&\\
	\bottomrule
\end{tabular}

    \end{adjustbox}
\end{table*}
%%%%%%%%

\begin{table*}[]
    \centering
    % \footnotesize
    % \fontsize{7}{7}
%    \renewcommand{\arraystretch}{0.6}
    \caption{Breakdown of the sample-level attack on four different ClinicalBERT models, using PubMed-BERT as the reference. Sample-level attack attempts to determine the membership of a single sample. In this table, i2b2 data is used as non-members in the target sample pool.}
    \vspace{-2ex}
    \label{tab:app:sample-i2b2}
    \begin{adjustbox}{width=\textwidth, center}
     \newcolumntype{L}{>{\RaggedLeft\arraybackslash}p{0.06\linewidth}} 
  \newcolumntype{O}{>{\RaggedLeft\arraybackslash}m{0.07\linewidth}} 
  \newcolumntype{D}{>{\arraybackslash}m{0.15\linewidth}} 
  \newcolumntype{R}{>{\arraybackslash}m{0.29\linewidth}} 
% \begin{tabular}{@{}cDrrrrrcrrrr@{}}
\begin{tabular}{@{}clSSSSScSSSSS@{}}
	\toprule
	& {\multirow{2}{*}{}} &  \multicolumn{4}{c}{{Short}}&{}& \multicolumn{4}{c}{{Long}}   \\
	\cmidrule{3-6} \cmidrule{8-11}
	&   &  {Base} & {Long} &  {Large} &{Large++}& {} & {Base} &{Long} & {Large}& {Large++}  \\
% 	&Metric &Original &A4NT	&One-LM	 &One-LM (DB25)	 &One-LM (DB40)	 &Inters.	&Inters. (DB25)	&Inters. (DB40)	&Union \\
	%%%%%%%%%
    \midrule
	%%%%%%%%%
    \multirow{2}{*}{\STAB{AUC.}} 
    &Baseline   & 75.6  &	75.0    &	77.6&	79.6&   	&81.2&	80.8&	82.8&	85.0	\\
    &Ours	    & 84.5  &	84.0    &	85.5&	86.7&   	&88.1&	88.0&	88.8&	89.7   \\
    %%%%%%%%%%&&&&&&&\\&&&&      &  & & &&&&&& &  & & && & &
           \midrule[0.1pt]
    \multirow{2}{*}{\STAB{Prec.}}
    &Baseline	& 69.9&	69.4&	72.1&	74.2&   &	77.9&	76.9&	79.0&	81.5   \\
    &Baseline 2 & 72.6&	72.0&	74.4&	76.4&   &	80.1&	79.3&	81.4&	83.2 \\ 
    &Ours	    & 92.5&	92.6&	92.3&	92.0&   &	94.7&	95.0&	94.3&	94.4   \\
    %%%%%%%%%%%&&&&&&&\\&&&&     &  & & &&&&&& &  & & && & &
           \midrule[0.1pt]
    \multirow{2}{*}{\STAB{Acc.}}
    &Baseline	&   55.5&	55.5&	56.2&	56.0&   &	54.8&	54.7&	55.0&	55.4  \\
    &Baseline 2 &   26.2&	25.4&	28.3&	31.5&   &	37.7&	38.0&	43.0&	48.7 \\
    &Ours	    &   43.7&	43.2&	45.7&	48.0&   &	50.0&	49.6&	51.8&	54.4    \\
    %%%%%%%%%%%&&&&&&&\\
	\bottomrule
\end{tabular}

    \end{adjustbox}
\end{table*}
%%%%%%%%

%%%%
\begin{table*}[]
    \centering
    % \footnotesize
    % \fontsize{7}{7}
%    \renewcommand{\arraystretch}{0.6}
    \caption{Breakdown of the patient-level attack on four different ClinicalBERT models, using PubMed-BERT as the reference. patient-level attack attempts to determine the membership of a patient based on all their samples. In this table the MIMIC-III heldout data  is used as non-members in the target sample pool.}
    \vspace{-2ex}
    \label{tab:app:patient-out}
    \begin{adjustbox}{width=\textwidth, center}
     \newcolumntype{L}{>{\RaggedLeft\arraybackslash}p{0.06\linewidth}} 
  \newcolumntype{O}{>{\RaggedLeft\arraybackslash}m{0.07\linewidth}} 
  \newcolumntype{D}{>{\arraybackslash}m{0.15\linewidth}} 
  \newcolumntype{R}{>{\arraybackslash}m{0.29\linewidth}} 
% \begin{tabular}{@{}cDrrrrrcrrrr@{}}

	%
\begin{tabular}{@{}clSSSSScSSSSS@{}}
	\toprule
	& {\multirow{2}{*}{}} &  \multicolumn{4}{c}{{Short}}&{}& \multicolumn{4}{c}{{Long}}   \\
	\cmidrule{3-6} \cmidrule{8-11}
	&   &  {Base} & {Long} &  {Large} &{Large++}& {} & {Base} &{Long} & {Large}& {Large++}  \\
% 	&Metric &Original &A4NT	&One-LM	 &One-LM (DB25)	 &One-LM (DB40)	 &Inters.	&Inters. (DB25)	&Inters. (DB40)	&Union \\
	%%%%%%%%%
    \midrule
	%%%%%%%%%
    \multirow{2}{*}{\STAB{AUC.}} 
    &Baseline   & 62.8&	60.5&	62.4&	66.8&&	91.5&	90.7&	94.1&	93.9	\\
    &Ours	    & 98.4&	98.8&	98.3&	97.8&&	99.2&	99.3&	99.3&	99.3  \\
    %%%%%%%%%%&&&&&&&\\&&&&      &  & & &&&&&& &  & & && & &
           \midrule[0.1pt]
    \multirow{2}{*}{\STAB{Prec.}}
    &Baseline	& 59.6&	59.3&	62.4&	63.4&&	88.2&	83.9&	94.2&	92.6   \\
    &Baseline 2 & 55.9&	55.9&	54.7&	54.7&&	62.3&	60.4&	60.4&	57.6 \\ 
    &Ours	    & 61.5&	61.9&	59.3&	57.9&&	81.8&	81.1&	79.2&	76.7  \\
    %%%%%%%%%%%&&&&&&&\\&&&&     &  & & &&&&&& &  & & && & &
           \midrule[0.1pt]
    \multirow{2}{*}{\STAB{Acc.}}
    &Baseline	&   53.5 &	54.5	&58.6&	52.5&&  45.5 &	47.5 &	49.5 &	50.5  \\
    &Baseline 2 &   100.0&	100.0&	100.0&	100.0&&	100.0&	100.0&	100.0&	100.0 \\
    &Ours	    &   100.0&	100.0&	100.0&	100.0&&	100.0&	100.0&	100.0&	100.0  \\
    %%%%%%%%%%%&&&&&&&\\
	\bottomrule
\end{tabular}

    \end{adjustbox}
\end{table*}
%%%%%%
\begin{table*}[]
    \centering
    % \footnotesize
    % \fontsize{7}{7}
%    \renewcommand{\arraystretch}{0.6}
    \caption{Breakdown of the patient-level attack on four different ClinicalBERT models, using PubMed-BERT as the reference. patient-level attack attempts to determine membership of a patient based on all their samples. In this table the i2b2  is used as non-members in the target sample pool.}
    \vspace{-2ex}
    \label{tab:app:patient-i2b2}
    \begin{adjustbox}{width=\textwidth, center}
     \newcolumntype{L}{>{\RaggedLeft\arraybackslash}p{0.06\linewidth}} 
  \newcolumntype{O}{>{\RaggedLeft\arraybackslash}m{0.07\linewidth}} 
  \newcolumntype{D}{>{\arraybackslash}m{0.15\linewidth}} 
  \newcolumntype{R}{>{\arraybackslash}m{0.29\linewidth}} 
% \begin{tabular}{@{}cDrrrrrcrrrr@{}}

	%
\begin{tabular}{@{}clSSSSScSSSSS@{}}
	\toprule
	& {\multirow{2}{*}{}} &  \multicolumn{4}{c}{{Short}}&{}& \multicolumn{4}{c}{{Long}}   \\
	\cmidrule{3-6} \cmidrule{8-11}
	&   &  {Base} & {Long} &  {Large} &{Large++}& {} & {Base} &{Long} & {Large}& {Large++}  \\
% 	&Metric &Original &A4NT	&One-LM	 &One-LM (DB25)	 &One-LM (DB40)	 &Inters.	&Inters. (DB25)	&Inters. (DB40)	&Union \\
	%%%%%%%%%
    \midrule
	%%%%%%%%%
    \multirow{2}{*}{\STAB{AUC.}} 
    &Baseline   & 100.0&	100.0&	100.0&	100.0&	&100.0	&100.0	&100.0	&100.0	\\
    &Ours	    & 100.0&	100.0&	100.0&	100.0&	&100.0	&100.0	&100.0	&100.0  \\
    %%%%%%%%%%&&&&&&&\\&&&&      &  & & &&&&&& &  & & && & &
           \midrule[0.1pt]
    \multirow{2}{*}{\STAB{Prec.}}
    &Baseline	& 100.0	&100.0&	100.0&	100.0&&	100.0  &	100.0&	100.0 &	100.0   \\
    &Baseline 2 & 94.3	&94.3	&97.1&	97.1	&&90.0 &	89.2	&86.1 &	83.2 \\ 
    &Ours	    & 95.2	&95.2	&93.4&	92.5	&&91.7 &	91.7	&90.0 &	90.8  \\
    %%%%%%%%%%%&&&&&&&\\&&&&     &  & & &&&&&& &  & & && & &
           \midrule[0.1pt]
    \multirow{2}{*}{\STAB{Acc.}}
    &Baseline	&   53.5 &	54.5	&58.6 &	52.5& &  45.5 &	47.5	&49.5&	50.5  \\
    &Baseline 2 &   100.0&	100.0&	100.0 &	100.0&&	100.0 &	100.0&	100.0&	100.0 \\
    &Ours	    &   100.0&	100.0&	100.0 &	100.0&&	100.0 &	100.0&	100.0&	100.0  \\
    %%%%%%%%%%%&&&&&&&\\
	\bottomrule
\end{tabular}

    \end{adjustbox}
\end{table*}
%%%%%%%%

%%%%%%%%
\begin{table*}[]
    \centering
    % \footnotesize
    % \fontsize{7}{7}
%    \renewcommand{\arraystretch}{0.6}
    \caption{Breakdown of the sample-level attack on ClinicalBERT-Base and Base-b (name insertion) models, using PubMed-BERT and standard bert-base-uncased as the references.  Sample-level attack attempts to determine membership of a single sample. In this table the MIMIC-III heldout data  is used as non-members in the target sample pool.}
    \vspace{-2ex}
    \label{tab:app:sample-out-b}
    \begin{adjustbox}{width=\textwidth, center}
     \newcolumntype{L}{>{\RaggedLeft\arraybackslash}p{0.06\linewidth}} 
  \newcolumntype{O}{>{\RaggedLeft\arraybackslash}m{0.07\linewidth}} 
  \newcolumntype{D}{>{\arraybackslash}m{0.15\linewidth}} 
  \newcolumntype{R}{>{\arraybackslash}m{0.29\linewidth}} 
% \begin{tabular}{@{}cDrrrrrcrrrr@{}}
\begin{tabular}{@{}clSSSSScSSSSS@{}}
	\toprule
	& {\multirow{2}{*}{}} &  \multicolumn{4}{c}{{Short}}&{}& \multicolumn{4}{c}{{Long}}   \\
	\cmidrule{3-6} \cmidrule{8-11}
	& {\multirow{2}{*}{}} &  \multicolumn{2}{c}{{Base}}&\multicolumn{2}{c}{{Base-1b}}&{}& \multicolumn{2}{c}{{Base}}& \multicolumn{2}{c}{{Base-1b}}   \\
		\cmidrule{3-4} \cmidrule{5-6} \cmidrule{8-9}\cmidrule{10-11}
	&   &  {Pubmed} & {Standard} &  {Pubmed} &{Standard}& {} & {Pubmed} &{Standard} & {Pubmed}& {Standard}  \\
% 	&Metric &Original &A4NT	&One-LM	 &One-LM (DB25)	 &One-LM (DB40)	 &Inters.	&Inters. (DB25)	&Inters. (DB40)	&Union \\
	%%%%%%%%%
    \midrule
	%%%%%%%%%
    \multirow{2}{*}{\STAB{AUC.}} 
    &Baseline   & 51.6&	51.6&	39.1&	39.1&			&66.2&	66.2&	56.1&	56.1	\\
    &Ours	    & 83.0&	80.6&	91.2&	83.1&			&90.0&	88.3&	96.0&	81.1   \\
    %%%%%%%%%%&&&&&&&\\&&&&      &  & & &&&&&& &  & & && & &
           \midrule[0.1pt]
    \multirow{2}{*}{\STAB{Prec.}}
    &Baseline	& 50.9&	50.9&	44.0&	44.0&			&61.5&	61.5&	52.8&	52.8   \\
    &Baseline 2 & 48.3&	48.3&	32.2&	32.2&			&61.5&	61.5&	49.3&	49.3 \\ 
    &Ours	    & 97.2&	91.9&	97.9&	93.2&			&99.0&	96.1&	99.5&	79.0  \\
    %%%%%%%%%%%&&&&&&&\\&&&&     &  & & &&&&&& &  & & && & &
           \midrule[0.1pt]
    \multirow{2}{*}{\STAB{Acc.}}
    &Baseline	&   55.4&	55.4&	52.1&	52.1&			&54.8&	54.8&	52.3&	52.3 \\
    &Baseline 2 &   26.2&	26.2&	12.9&	12.9&			&37.9&	37.9&	20.6&	20.6 \\
    &Ours	    &   44.1&	44.4&	59.3&	47.3&			&50.9&	49.7&	68.8&	57.5    \\
    %%%%%%%%%%%&&&&&&&\\
	\bottomrule
\end{tabular}

    \end{adjustbox}
\end{table*}
%%%%%%%%
%%%%%%%%
\begin{table*}[]
    \centering
    % \footnotesize
    % \fontsize{7}{7}
%    \renewcommand{\arraystretch}{0.6}
    \caption{Breakdown of the sample-level attack on ClinicalBERT-Base and Base-b (name insertion) models, using PubMed-BERT and standard bert-base-uncased as the references.  Sample-level attack attempts to determine membership of a single sample. In this table the i2b2 data  is used as non-members in the target sample pool.}
    \vspace{-2ex}
    \label{tab:app:sample-i2b2-b}
    \begin{adjustbox}{width=\textwidth, center}
     \newcolumntype{L}{>{\RaggedLeft\arraybackslash}p{0.06\linewidth}} 
  \newcolumntype{O}{>{\RaggedLeft\arraybackslash}m{0.07\linewidth}} 
  \newcolumntype{D}{>{\arraybackslash}m{0.15\linewidth}} 
  \newcolumntype{R}{>{\arraybackslash}m{0.29\linewidth}} 
% \begin{tabular}{@{}cDrrrrrcrrrr@{}}
\begin{tabular}{@{}clSSSSScSSSSS@{}}
	\toprule
	& {\multirow{2}{*}{}} &  \multicolumn{4}{c}{{Short}}&{}& \multicolumn{4}{c}{{Long}}   \\
	\cmidrule{3-6} \cmidrule{8-11}
	& {\multirow{2}{*}{}} &  \multicolumn{2}{c}{{Base}}&\multicolumn{2}{c}{{Base-1b}}&{}& \multicolumn{2}{c}{{Base}}& \multicolumn{2}{c}{{Base-1b}}   \\
		\cmidrule{3-4} \cmidrule{5-6} \cmidrule{8-9}\cmidrule{10-11}
	&   &  {Pubmed} & {Standard} &  {Pubmed} &{Standard}& {} & {Pubmed} &{Standard} & {Pubmed}& {Standard}  \\
% 	&Metric &Original &A4NT	&One-LM	 &One-LM (DB25)	 &One-LM (DB40)	 &Inters.	&Inters. (DB25)	&Inters. (DB40)	&Union \\
	%%%%%%%%%
    \midrule
	%%%%%%%%%
    \multirow{2}{*}{\STAB{AUC.}} 
    &Baseline   & 75.6&	75.6&	65.1&	65.1&			&81.2&	81.2&	71.8&	71.8	\\
    &Ours	    & 84.5&	80.3&	91.2&	85.7&			&88.1&	89.1&	94.3&	91.0   \\
    %%%%%%%%%%&&&&&&&\\&&&&      &  & & &&&&&& &  & & && & &
           \midrule[0.1pt]
    \multirow{2}{*}{\STAB{Prec.}}
    &Baseline	& 69.9&	70.0&	60.0&	60.0&			&77.9&	77.9&	66.0&	66.0   \\
    &Baseline 2 & 72.6&	72.6&	56.5&	56.5&			&80.1&	80.1&	67.8&	67.8 \\ 
    &Ours	    & 92.5&	85.8&	94.4&	90.4&			&94.7&	97.4&	96.2&	94.6  \\
    %%%%%%%%%%%&&&&&&&\\&&&&     &  & & &&&&&& &  & & && & &
           \midrule[0.1pt]
    \multirow{2}{*}{\STAB{Acc.}}
    &Baseline	&   55.5&	55.6&	51.8&	51.8&			&54.8&	54.8&	52.0&	52.0\\
    &Baseline 2 &   26.2&	26.3&	12.7&	12.7&			&37.7&	37.7&	20.1&	20.1\\
    &Ours	    &   43.7&	30.5&	59.1&	46.7&			&50.0&	49.4&	68.4&	57.0    \\
    %%%%%%%%%%%&&&&&&&\\
	\bottomrule
\end{tabular}

    \end{adjustbox}
\end{table*}
%%%%%%%%

%\subsection{Loss Distribution Visualizations}

\begin{figure}[t]
    \centering
        \begin{subfigure}{0.6\textwidth}
     \includegraphics[width=\linewidth]{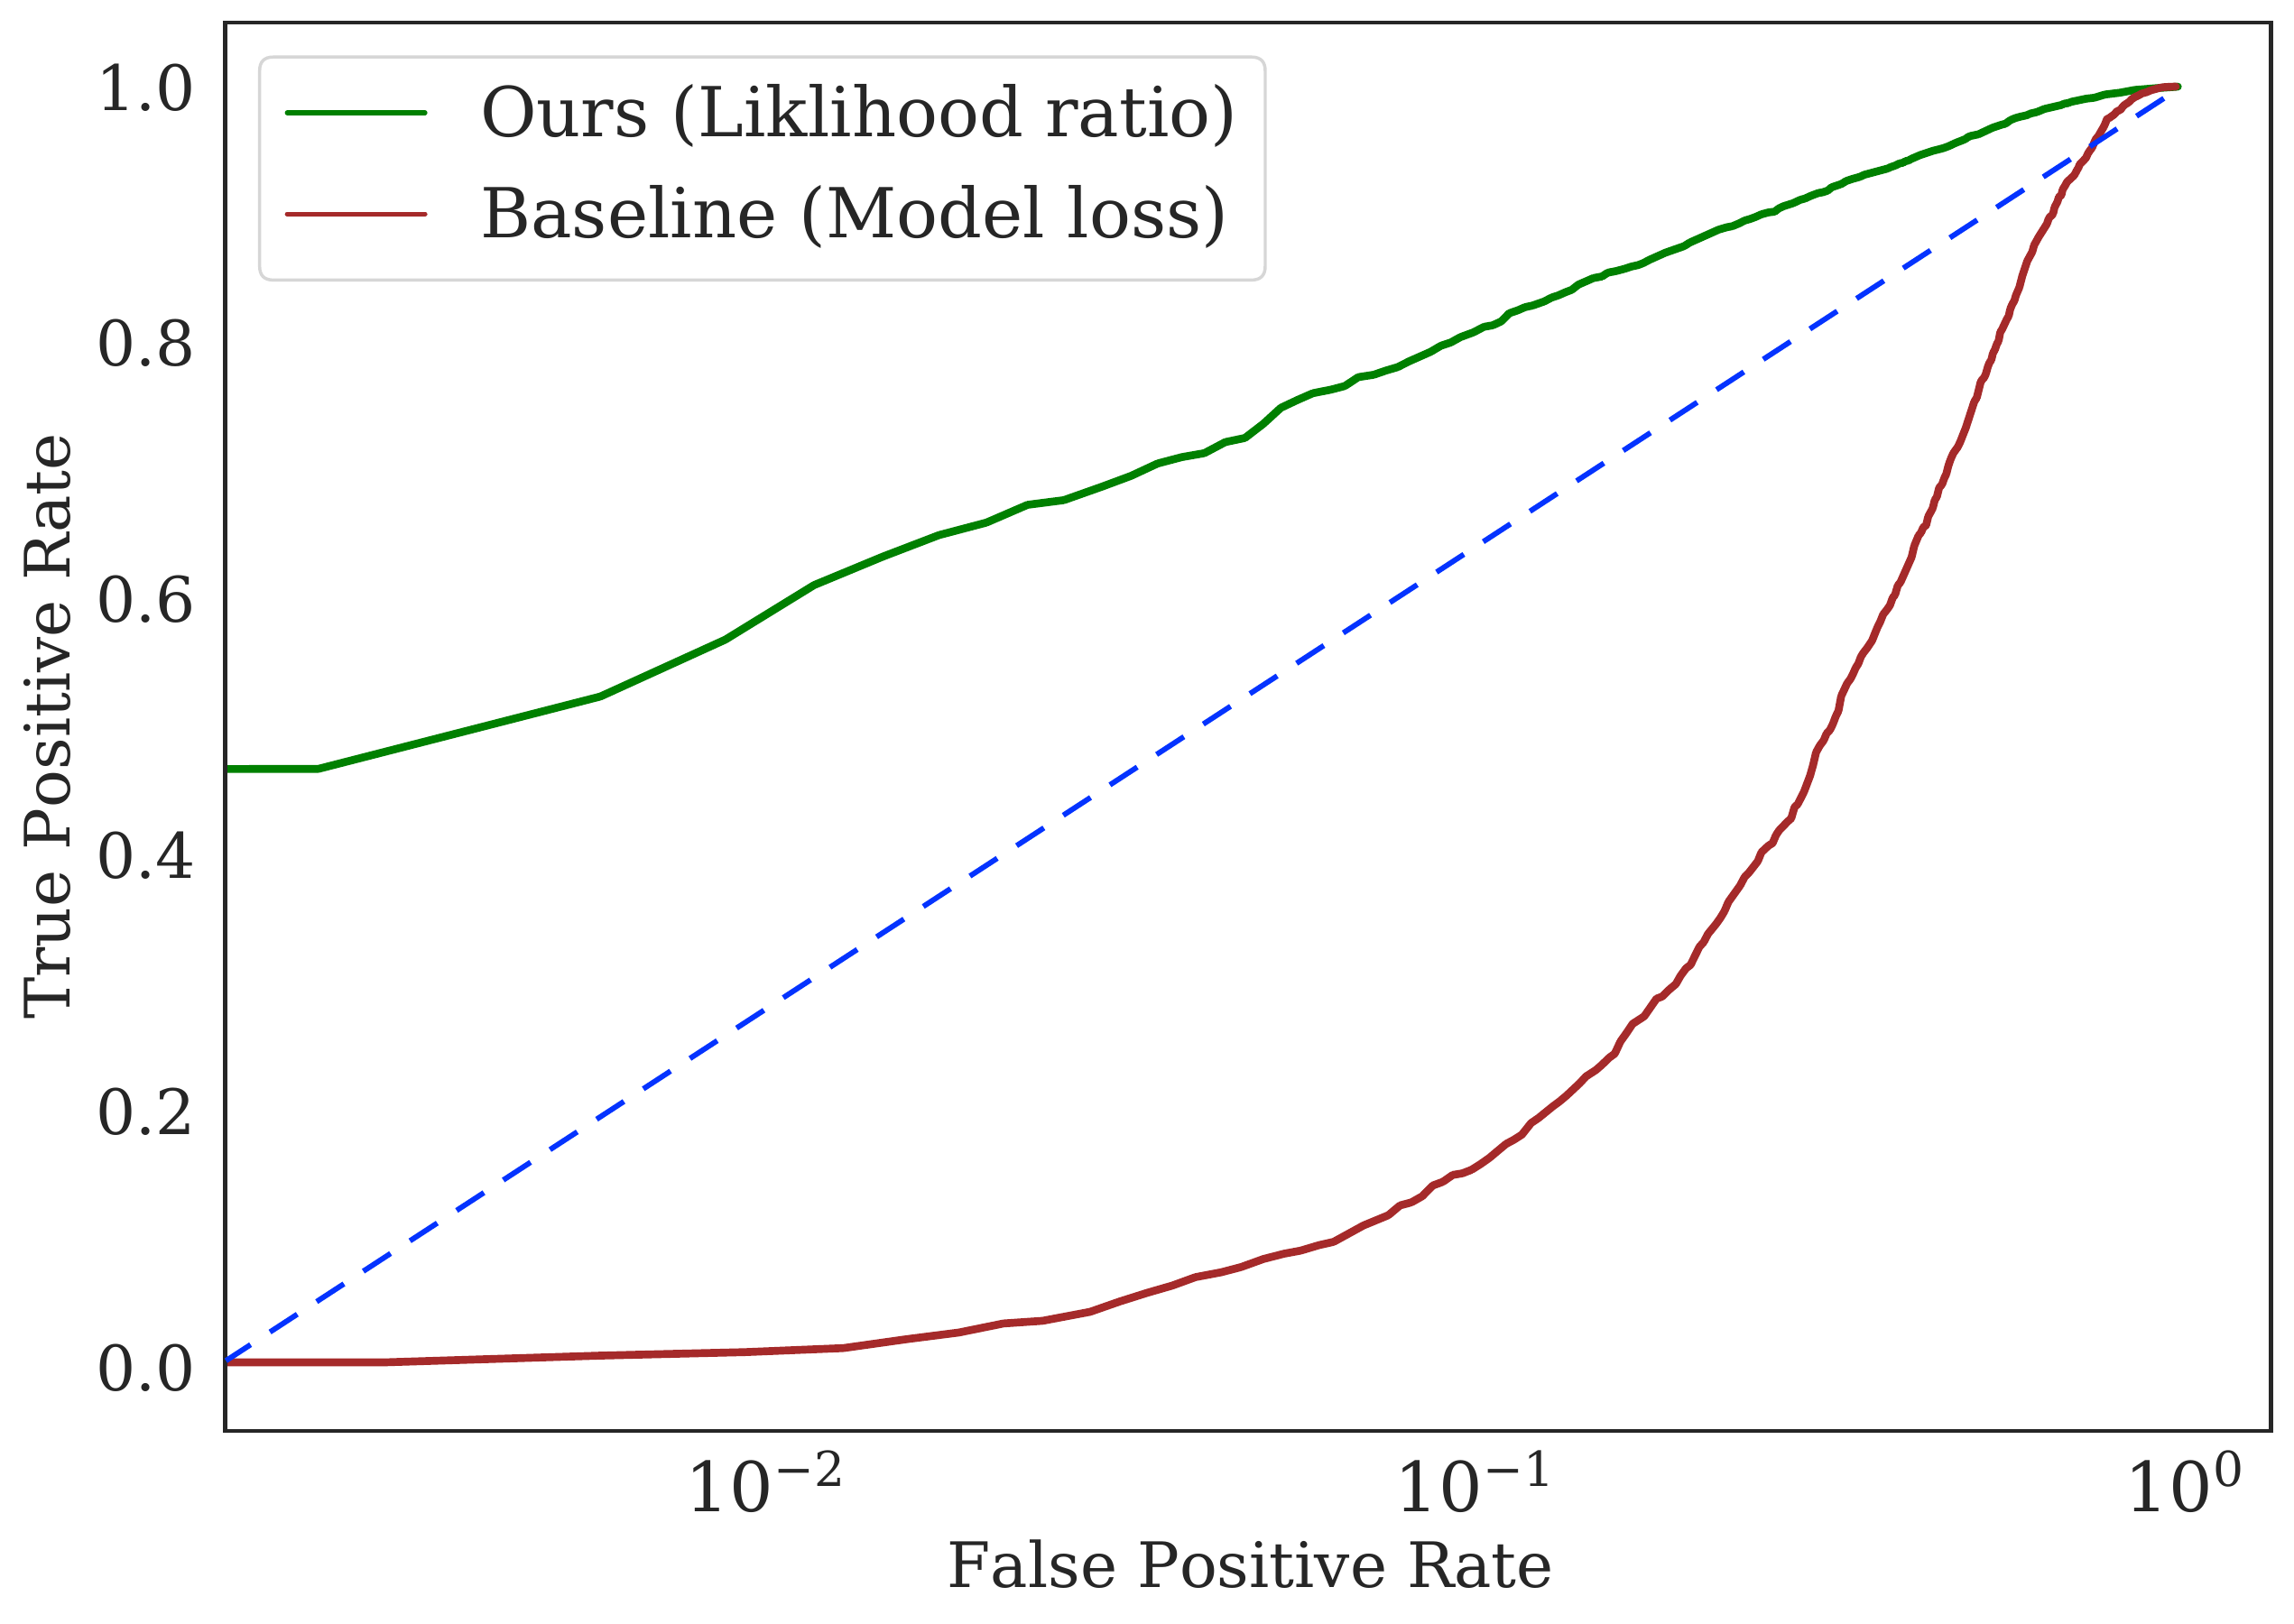}
    \footnotesize 
    \end{subfigure}
    % \begin{subfigure}{0.28\textwidth}
    %  \includegraphics[width=\linewidth]{figs/mnist_dpsgd_15.png}
    %  \caption{MNIST DP-SGD for $\varepsilon=15$}
    %  \label{fig:blogs-2dom-unc}
    % \end{subfigure}
    \caption{The ROC curve of sample-level attack, with logarithmic scale x-axis. performed on Clinical-BERT using MIMIC samples as non-members.  Green line shows our attack and  the red line shows the baseline loss-based attack. The blue dashed line shows AUC=$0.5$ (random uess). We find false positive and true positive rates over the target sample pool, which is comprised of members and non-members. }
    \label{fig:result:roc-log}
    \vspace{-2ex}
\end{figure}

%\rs{add a table of notations in the appendix}
\subsection{Notations}
To summarize and clarify the notations used in the paper for explaining our attack, we added Table~\ref{tab:attack_notation}.

\subsection{Breakdown of All Results}
Here, we have shown the full tables for each result presented in the body of the paper. In other words, we show all the results on both short and long samples, with both MIMIC-III and i2b2 datasets used as non-member samples. Tables~\ref{tab:app:sample-i2b2} and ~\ref{tab:app:sample-out-len} correspond to the sample-level i2b2 and MIMIC columns of Table~\ref{tab:overview-1b} and include all models from Table~\ref{tab:sample-out-len}. Similarly,  Tables~\ref{tab:app:patient-i2b2} and ~\ref{tab:app:patient-out} correspond to the patient-level column of Table~\ref{tab:overview}, and present results for all models from~\ref{tab:sample-out-len}. 

Finally, the last two Tables~\ref{tab:app:sample-i2b2-b} and~\ref{tab:app:sample-out-b}, breaks down the results in Table~\ref{tab:overview-1b}, which mainly revolve around the ClinicalBERT-b model (name insertion), on a sample level. 

In Figure~\ref{fig:result:roc-log} We have  plotted Figure~\ref{fig:result:roc} from the results, but with logarithmic x-axis, to zoom in on the low false positive rate section and really show the differences between our attack and the baseline.
